# Supplementary material for: Extracing the number of short-range corerlated nucleon pairs from inclusive electron scattering data
Source: arXiv:2005.01621 ancillary file (2021-02-24)
Supplement: Supplementary file 1 [file Sup_Figures_PRL.pdf]

# Study of inclusive electron scattering scaling using the generalized contact formalism: supplementary materials

## Figure 2 of the main text, for different nuclei and interactions:

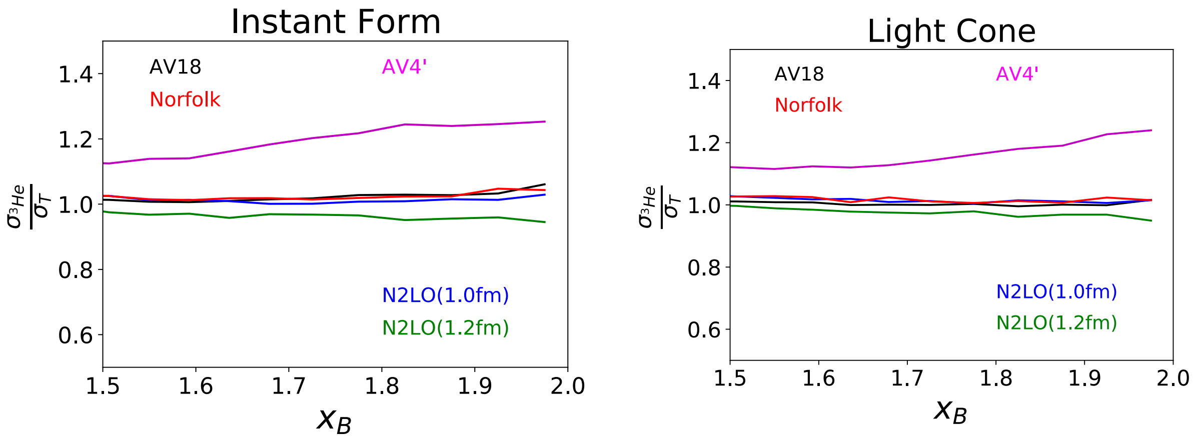


**Fig. S1:** Same as figure 2-left for $^3$He/$^3$H with Instant Form (left) and Light Cone (right). (contacts from Rey, E* = 0; $\sigma_{CM}$ = 60±10)

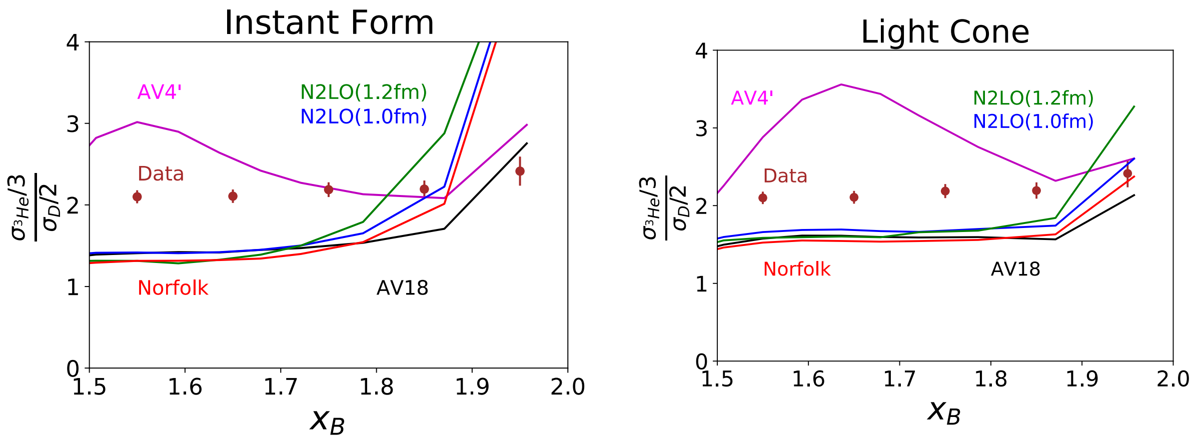


**Fig. S2:** Same as figure 2-top for $^3$He/d with Instant Form (left) and Light Cone (right) , compared with the data of Fomin et al.

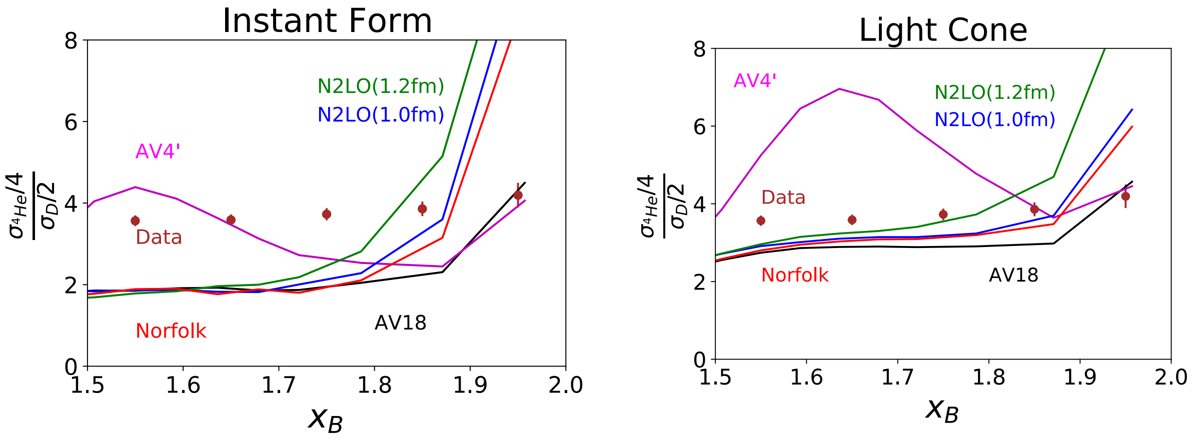


**Fig. S3:** Same as figure 2-top for $^4$He/d with Instant Form (left) and Light Cone (right) , compared with the data of Fomin et al.

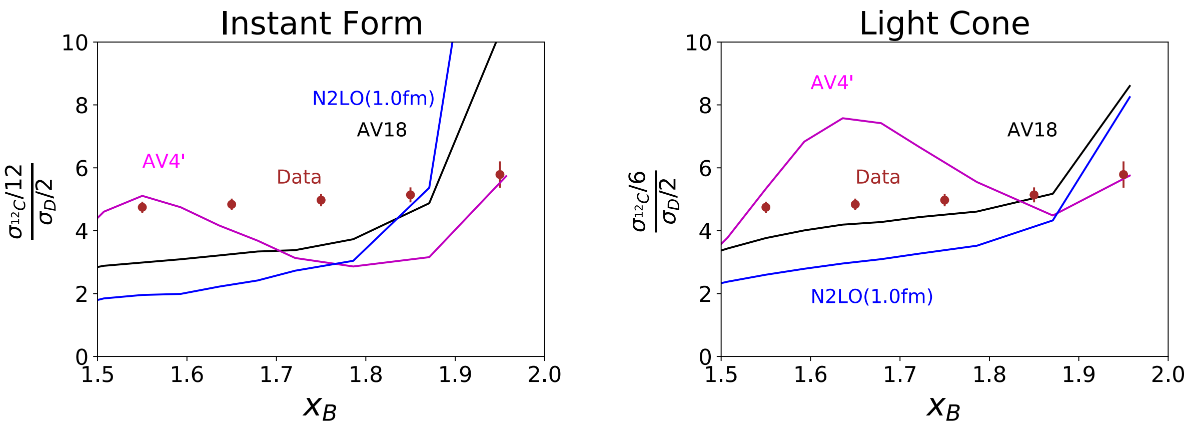


**Fig. S4:** Same as figure 2-top for $^{12}$C/d with Instant Form (left) and Light Cone (right), compared with the data of Fomin et al.

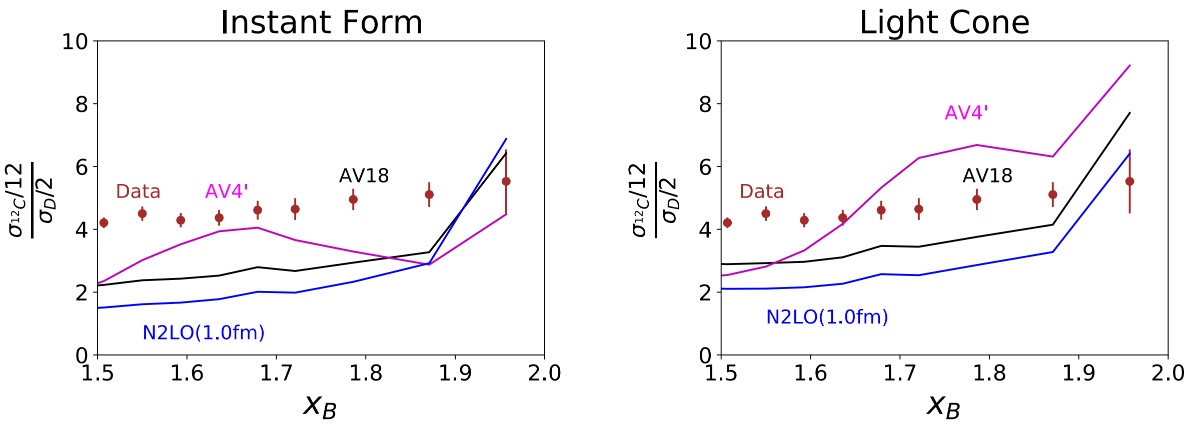


**Fig. S5:** Same as figure 2-top for $^{12}$C/d with Instant Form (left) and Light Cone (right), compared with the data of Schmookler et al.

## Fitting procedure:

The GCF parameters were inferred from the measured cross-section ratios using Maximum Likelihood Estimations (MLE). In this analysis there are three parameters of interest $C_{pn}^1, \sigma_{CM}$ and $E^*$. We assume that the uncertainties on the data represent Gaussian errors; therefore, out likelihood is calculated as:

$$\log\left(\mathcal{L}(C_{np}^1, \sigma_{CM}, E^*)\right) = -\sum_i \frac{\left(O\left(x_B^i \middle| C_{np}^1, \sigma_{CM}, E^*\right) - E\left(x_B^i\right)\right)^2}{2\sigma(x_B^i)^2}$$

$\mathcal{L}$ is the likelihood of a set of parameters. $E(x_{Bi})$ is the set of experimental data points used in the fit where $x_B^i$ corresponds to $x_B$ at bin i and $E$ corresponds to the cross section ratio. $\sigma(x_B^i)$ is the experimental error of the data point at $x_B^i$. $O\left(x_B^i \middle| C_{pn}^1, \sigma_{CM}, E^*\right)$ is the cross section ratio calculated with the GCF for the given set of parameters.

$$O\left(x_B^i \middle| C_{np}^1, \sigma_{CM}, E^*\right) = \frac{\sigma_A\left(x_B^i \middle| C_{np}^1, \sigma_{CM}, E^*\right)/A}{\sigma_d(x_B^i)/2}$$

The log likelihood is maximized with respect to the parameters to determine their most likely value.

To estimate the confidence interval of each parameter the 1-dimensional likelihood of each parameter was first calculated by maximizing the likelihood with respect to all other parameters. For example, the likelihood for $C_{pn}^1$ is:

$$\log\left(\mathcal{L}(C_{np}^1)\right) = \max_{E^*, \sigma_{CM}} \left[\log\left(\mathcal{L}(C_{np}^1, \sigma_{CM}, E^*)\right)\right]$$

The most likely value of $C_{np}^1$ is at the maximum of $\log\left(\mathcal{L}(C_{np}^1)\right)$. The values of $C_{np}^1$ which satisfy:

$$\log\left(\mathcal{L}(C_{np}^1)\right) > \max[\log\left(\mathcal{L}(C_{np}^1, \sigma_{CM}, E^*)\right)] - \Delta \log \mathcal{L}$$

Are considered to be within the confidence region. For the 1-dimensional case at 68.3% confidence $\Delta \log \mathcal{L} = 0.5$. The same calculations can be applied to $\sigma_{CM}$ and $E^*$ to determine their most likely values and errors.

To create the 2-dimensional confidence interval, the likelihood is maximized only for the one remaining parameter. In the case of estimating the confidence interval for $C_{np}^1$ and $\sigma_{CM}$, $E^*$ is maximized.

$$\log(\mathcal{L}(C, \sigma_{CM})) = \max_{E^*}[\log(\mathcal{L}(C, \sigma_{CM}, E^*))]$$

The delta log likelihood is again used to determine the bounds. All points which satisfy:

$$\log(\mathcal{L}(C, \sigma_{CM})) > \max[\log\left(\mathcal{L}(C_{np}^1, \sigma_{CM}, E^*)\right)] - \Delta \log \mathcal{L}$$

Lie within the 2-dimensional confidence region. In the case of 2-dimensions and 68.3% confidence $\Delta \log \mathcal{L} = 1.15$. For 2-dimensions and 95.5% confidence $\Delta \log \mathcal{L} = 2.31$. We exclude from the fit the highest $x_B$ data point as it is very close to the kinematical limit of deuterium

## Table I of the main text, including additional nuclei and interactions:

| Data Set | | | $a_2(A/d)$ | $C_{np}^{s=1}(A/d)$ | $\sigma_{CM}$ $[MeV/c]$ | $E_{A-2}^{*}$ $[MeV]$ |
|---|---|---|---|---|---|---|
| $^{3}He$ Fomin | Experiment | | $2.14 \pm 0.04$ | - | $60 \pm 10$ | - |
| | AV18 | Ab-Initio | | $1.31 \pm 0.13$ | - | - |
| | | IF Fit | | $1.86^{+0.04}_{-0.04}$ | $36^{+15}_{-28}$ | 0 |
| | | LC Fit | | $1.78^{+0.04}_{-0.09}$ | $< 87$ | 0 |
| | AV4' | Ab-Initio | | $1.26 \pm 0.13$ | - | - |
| | | IF Fit | | $1.01^{+0.04}_{-0.04}$ | $< 8$ | 0 |
| | | LC Fit | | $0.93^{+0.04}_{-0.04}$ | $30^{+6}_{-5}$ | 0 |
| | N2LO (1.0fm) | Ab-Initio | | $1.43 \pm 0.15$ | - | - |
| | | IF Fit | | $2.14^{+0.05}_{-0.04}$ | $< 24$ | 0 |
| | | LC Fit | | $1.93^{+0.04}_{-0.20}$ | $< 78$ | 0 |
| | N2LO (1.2fm) | Ab-Initio | | $1.35 \pm 0.17$ | - | - |
| | | IF Fit | | $2.28^{+0.05}_{-0.07}$ | $15^{+4}_{-6}$ | 0 |
| | | LC Fit | | $1.74^{+0.20}_{-0.08}$ | $< 66$ | 0 |
| | Norfolk | Ab-Initio | | $1.27 \pm 0.18$ | - | - |
| | | IF Fit | | $2.05^{+0.05}_{-0.05}$ | <22 | 0 |
| | | LC Fit | | $1.88^{+0.04}_{-0.20}$ | $< 77$ | 0 |
| $^{4}He$ Fomin | Experiment | | $3.66 \pm 0.07$ | - | $100 \pm 20$ | - |
| | AV18 | Ab-Initio | | $2.58 \pm 0.26$ | - | - |
| | | IF Fit | | $4.16^{+1.04}_{-0.10}$ | $83^{+25}_{-9}$ | $< 19$ |
| | | LC Fit | | $3.22^{+0.21}_{-0.10}$ | $110^{+20}_{-15}$ | N/A |
| | AV4' | Ab-Initio | | $2.57 \pm 0.27$ | - | - |
| | | IF Fit | | $0.91^{+0.05}_{-0.05}$ | $62^{+5}_{-5}$ | 0 |
| | | LC Fit | | $1.97^{+0.05}_{-0.05}$ | $< 36$ | $< 4$ |
| | N2LO (1.0fm) | Ab-Initio | | $2.64 \pm 0.29$ | - | - |
| | | IF Fit | | $4.94^{+0.37}_{-0.16}$ | $54^{+6}_{-4}$ | $< 6$ |
| | | LC Fit | | $3.24^{+0.21}_{-0.11}$ | $90^{+16}_{-10}$ | N/A |
| | N2LO (1.2fm) | Ab-Initio | | $2.46 \pm 0.52$ | - | - |
| | | IF Fit | | $5.65^{+0.35}_{-0.15}$ | $41^{+3}_{-3}$ | $< 4$ |
| | | LC Fit | | $3.12^{+0.20}_{-0.10}$ | $77^{+9}_{-9}$ | N/A |
| | Norfolk | Ab-Initio | | $2.64 \pm 0.38$ | - | - |
| | | IF Fit | | $4.89^{+0.48}_{-0.16}$ | $59^{+7}_{-4}$ | $< 7$ |
| | | LC Fit | | $3.24^{+0.21}_{-0.11}$ | $89^{+19}_{-8}$ | N/A |
| $^{12}C$ Fomin | Experiment | | $4.88 \pm 0.10$ | - | $143 \pm 5$ | - |
| | AV18 | Ab-Initio | | $3.33 \pm 0.37$ | - | - |
| | | IF Fit | | $5.18^{+0.95}_{-0.20}$ | $75^{+20}_{-7}$ | $< 18$ |
| | | LC Fit | | $4.48^{+0.15}_{-0.50}$ | $124^{+10}_{-34}$ | N/A |
| | AV4' | Ab-Initio | | $2.3 \pm 0.24$ | - | - |
| | | IF Fit | | $2.26^{+0.01}_{-0.01}$ | $170^{+1}_{-1}$ | 0 |
| | | LC Fit | | $2.29^{+0.03}_{-0.03}$ | $40^{+1}_{-1}$ | $< 3$ |
| | N2LO (1.0fm) | Ab-Initio | | $2.27 \pm 0.23$ | - | - |
| | | IF Fit | | $6.26^{+0.48}_{-0.17}$ | $46^{+8}_{-5}$ | $< 7$ |
| | | LC Fit | | $4.42^{+0.14}_{-0.48}$ | $106^{+7}_{-27}$ | N/A |

| | | | | | | |
|---|---|---|---|---|---|---|
| $^{12}C$ Schmookler | Experiment | | $4.49 \pm 0.17$ | - | $143 \pm 5$ | - |
| | AV18 | Ab-Initio | | $3.33 \pm 0.37$ | - | - |
| | | IF Fit | | $7.90^{+2.75}_{-2.61}$ | $134^{+37}_{-38}$ | N/A |
| | | LC Fit | | $4.55^{+0.40}_{-0.13}$ | $103^{+41}_{-10}$ | N/A |
| | AV4' | Ab-Initio | | $2.3 \pm 0.24$ | - | - |
| | | IF Fit | | $5.07^{+0.74}_{-1.34}$ | $155^{+4}_{-32}$ | $> 26$ |
| | | LC Fit | | $4.01^{+0.14}_{-0.14}$ | $65^{+4}_{-6}$ | $> 59$ |
| | N2LO (1.0fm) | Ab-Initio | | $2.27 \pm 0.23$ | - | - |
| | | IF Fit | | $6.01^{+2.14}_{-0.50}$ | $88^{+33}_{-10}$ | $< 45$ |
| | | LC Fit | | $4.37^{+0.23}_{-0.18}$ | $101^{+31}_{-11}$ | N/A |

# Figure 3 of the main text, for different nuclei and interactions:

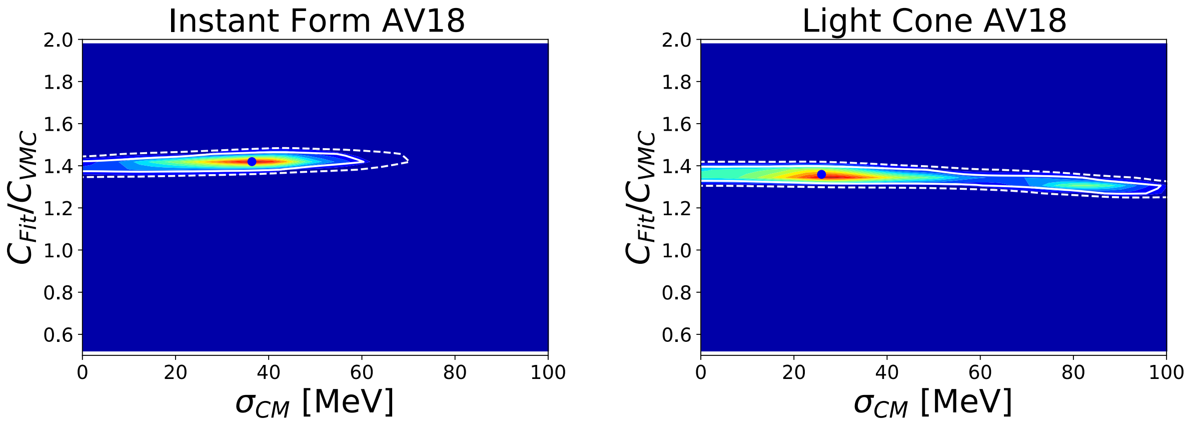


**Fig. S6:** Same as figure 3 for $^{3}$He using the AV18 potential and the data of Fomin et al.

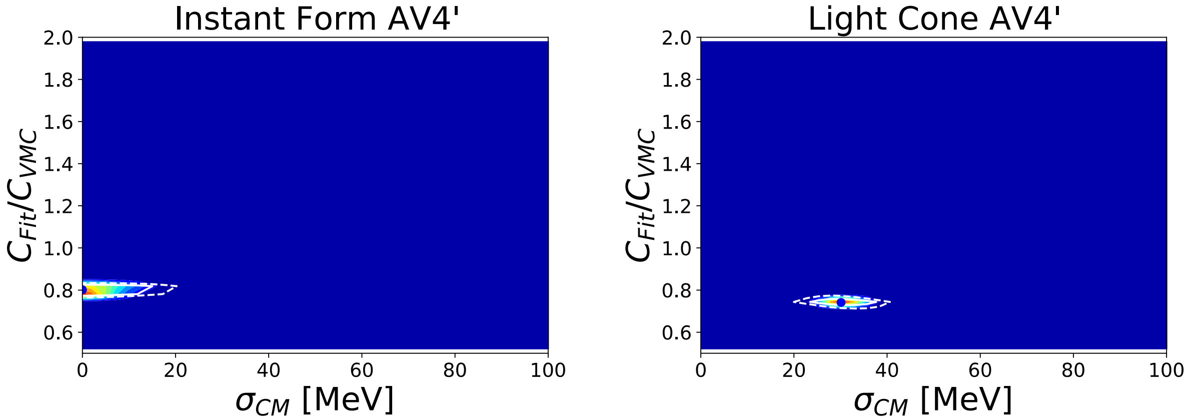


**Fig. S7:** Same as figure 3 for $^{3}$He using the AV4' potential and the data of Fomin et al.

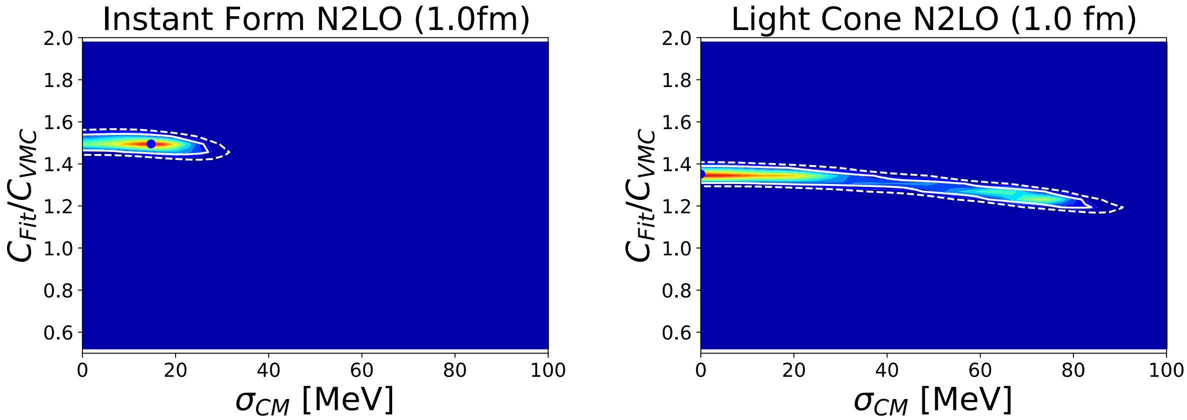


**Fig. S8:** Same as figure 3 for $^{3}$He using the N2LO(1.0fm) potential and the data of Fomin et al.

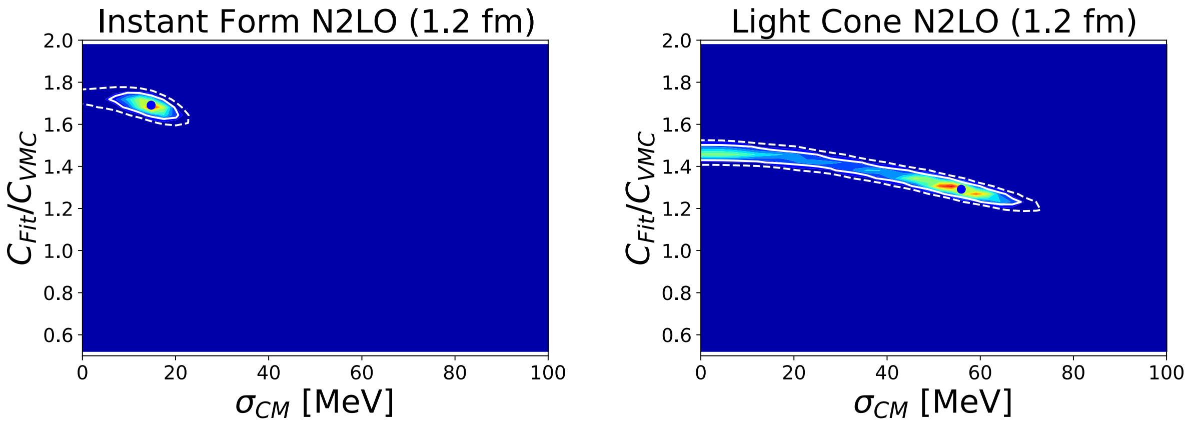


**Fig. S9:** Same as figure 3 for $^{3}He$ using the N2LO(1.2fm) potential and the data of Fomin et al.

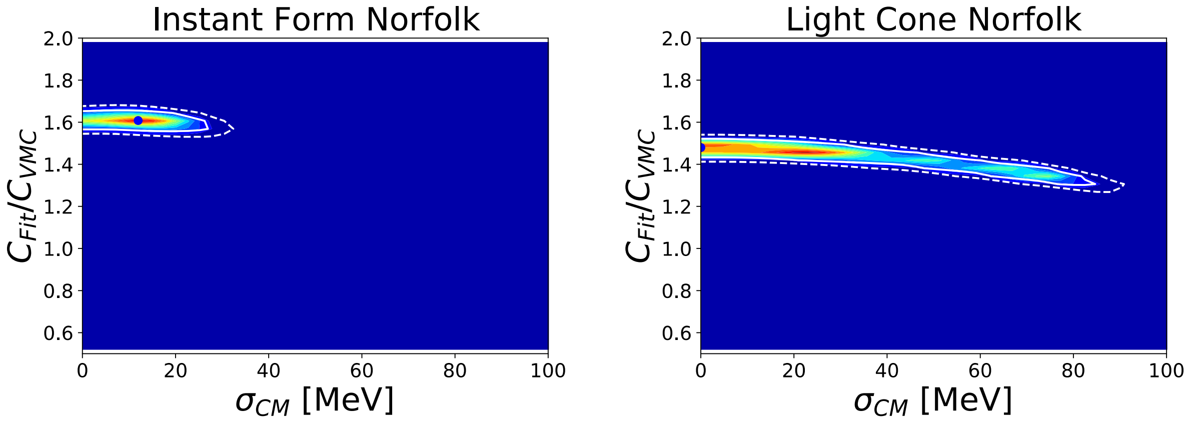


**Fig. S10:** Same as figure 3 for $^{3}He$ using the Norfolk potential and the data of Fomin et al.

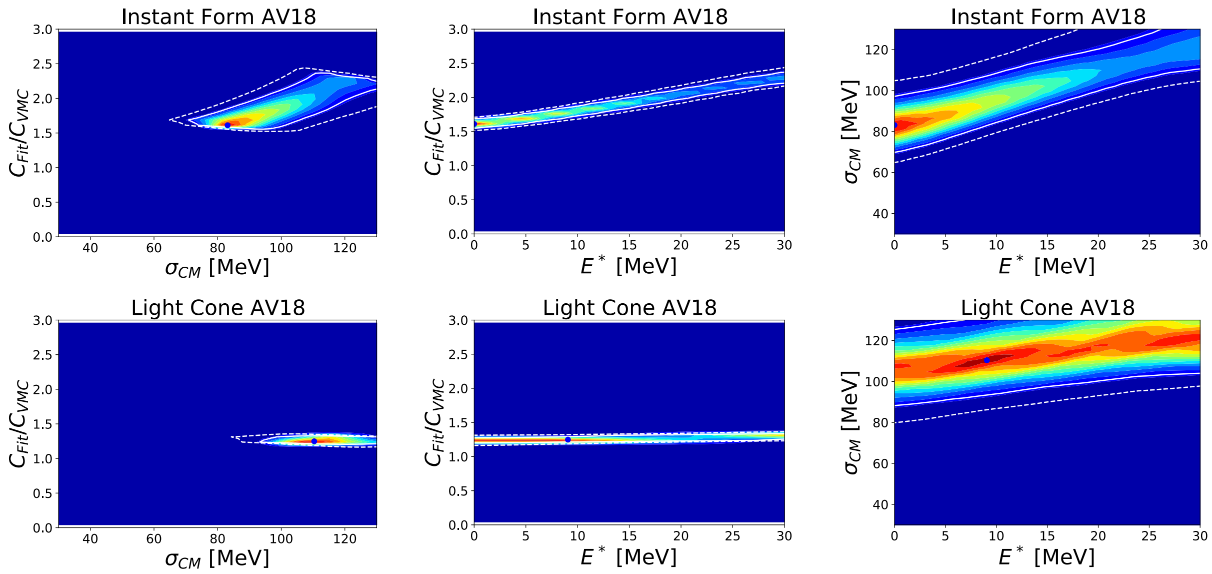


**Fig. S11:** Same as figure 3 for $^4$He using the AV18 potential and the data of Fomin et al.

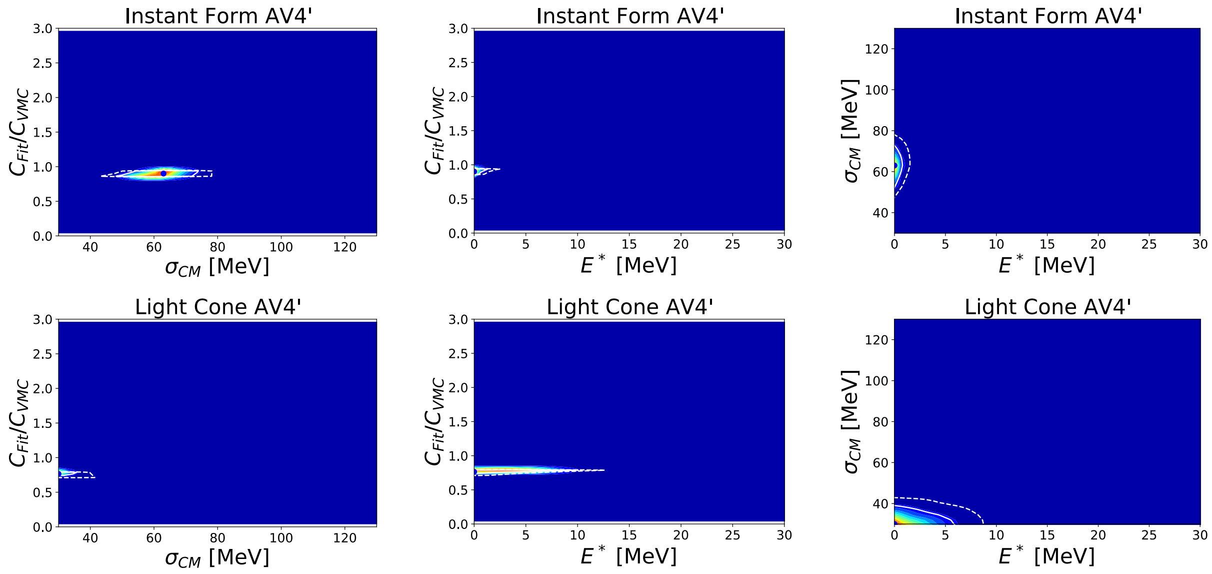


**Fig. S12:** Same as figure 3 for $^4$He using the AV4' potential and the data of Fomin et al.

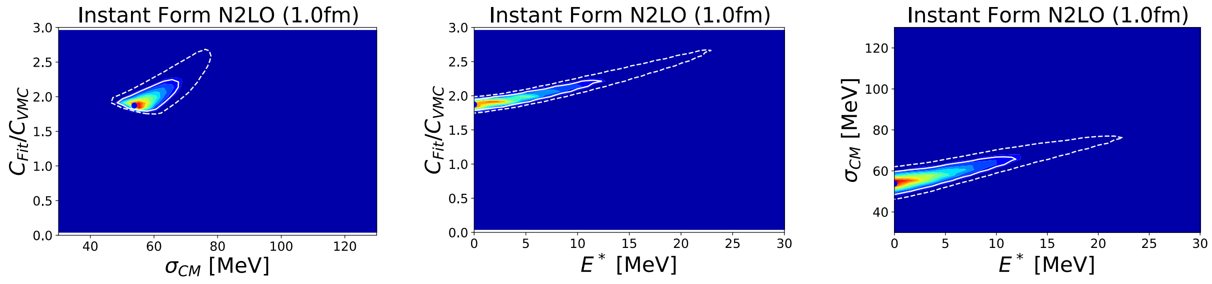

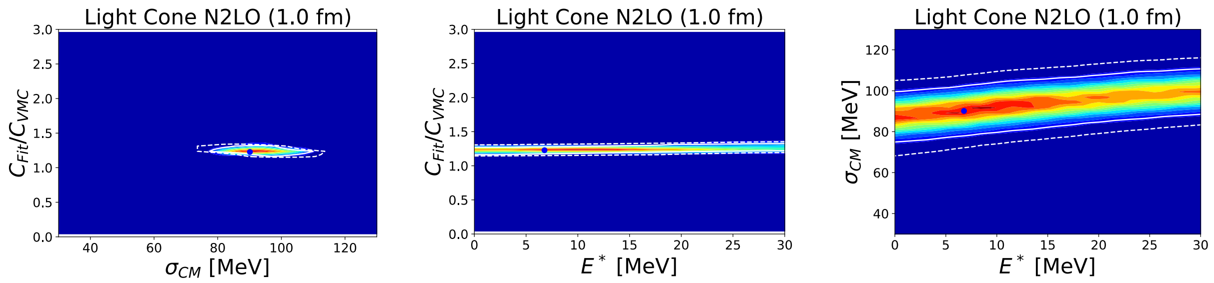


**Fig. S13:** Same as figure 3 for $^4$He using the N2LO(1.0fm) potential and the data of Fomin et al.

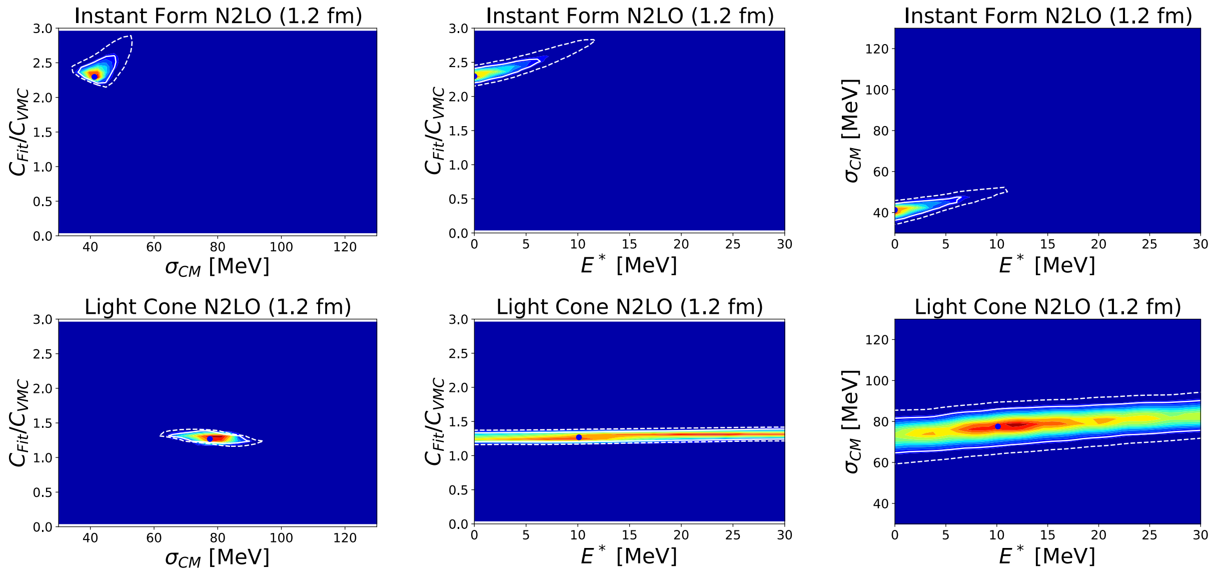


**Fig. S14:** Same as figure 3 for $^4$He using the N2LO(1.2fm) potential and the data of Fomin et al.

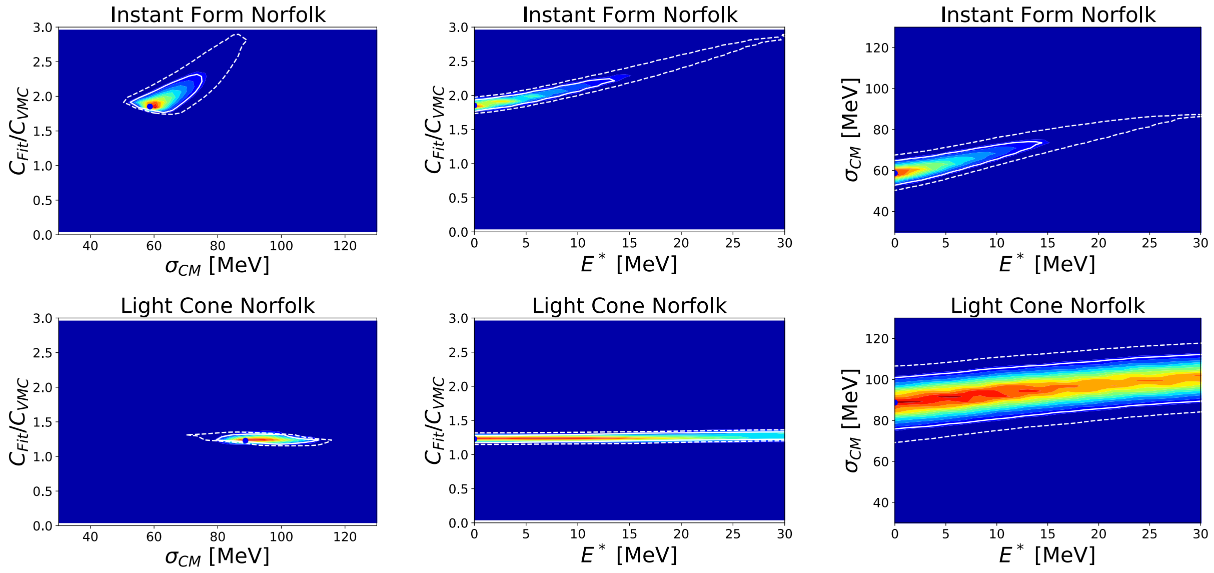


**Fig. S15:** Same as figure 3 for $^4$He using the Norfolk potential and the data of Fomin et al.

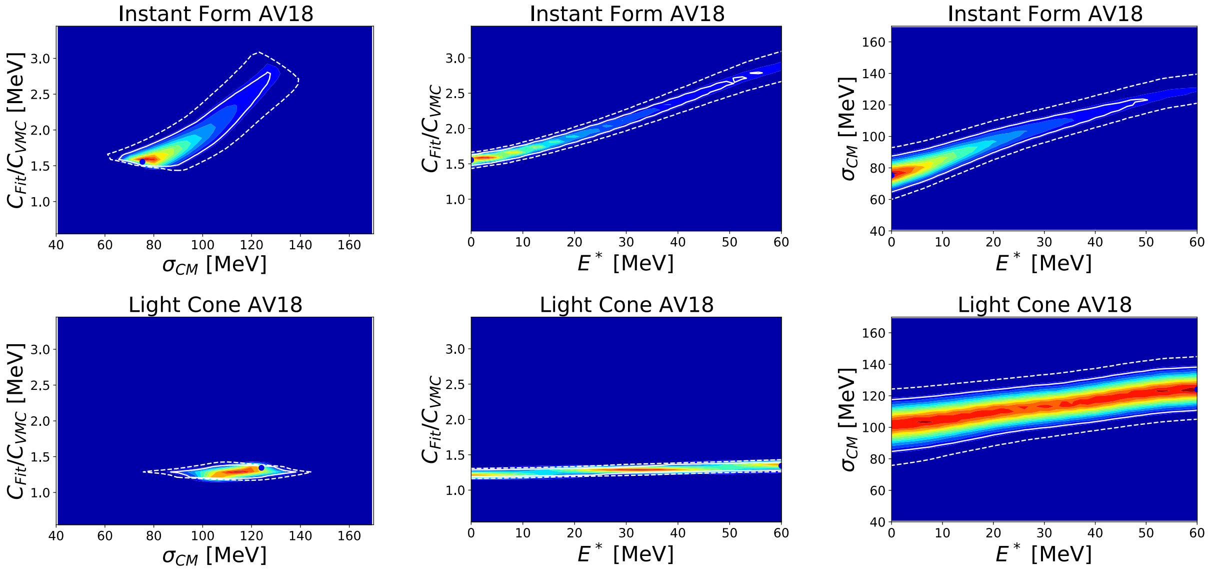


**Fig. S16:** Same as figure 3 for $^{12}C$ using the AV18 potential and the data of Fomin et al.

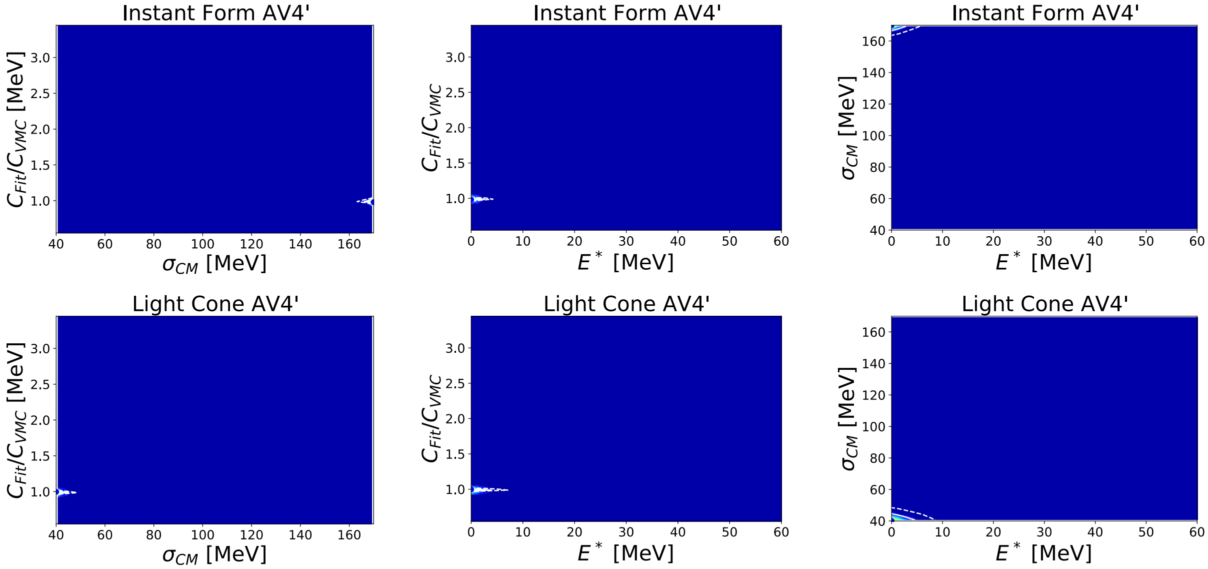


**Fig. S17:** Same as figure 3 for $^{12}C$ using the AV4' potential and the data of Fomin et al.

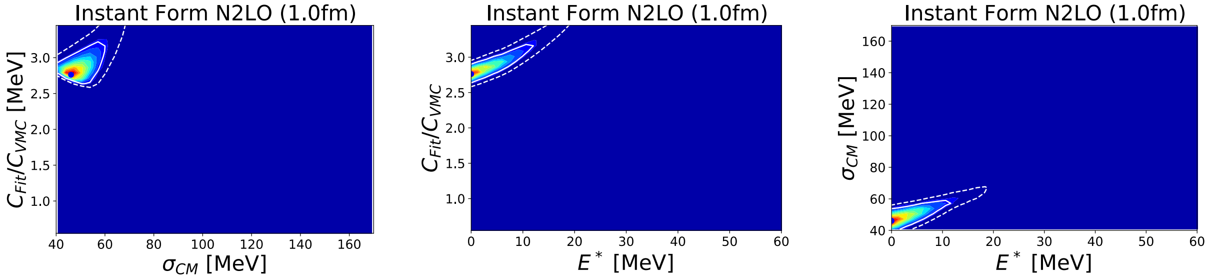

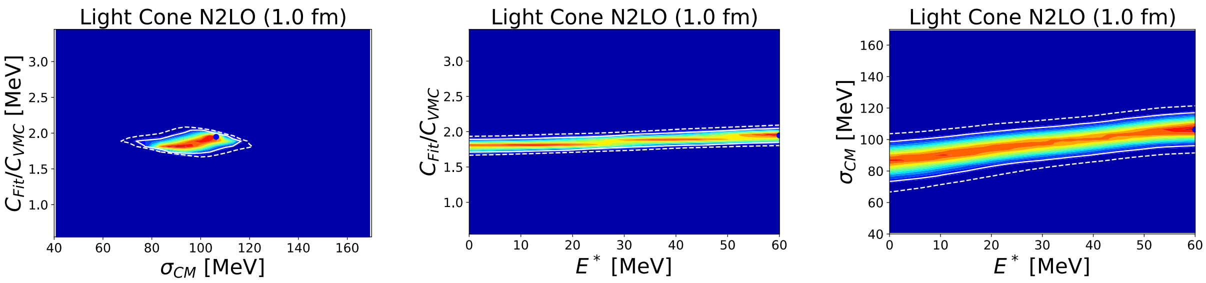


**Fig. S18:** Same as figure 3 for $^{12}$C using the N2LO(1.0fm) potential and the data of Fomin et al.

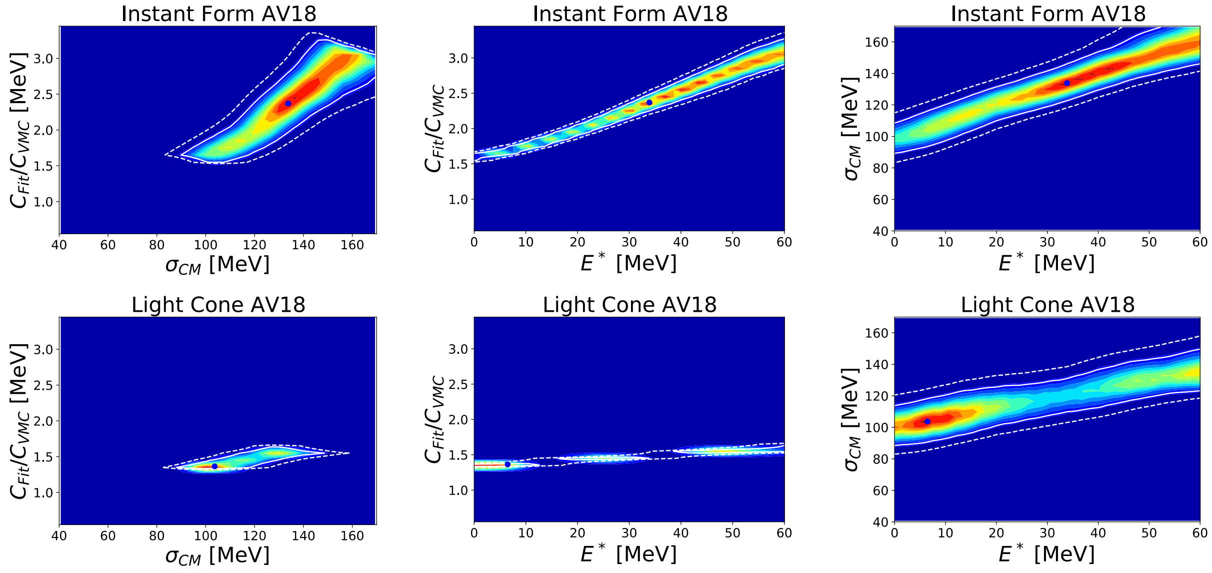


**Fig. S19:** Same as figure 3 for $^{12}$C using the AV18 potential and the data of Schmookler et al.

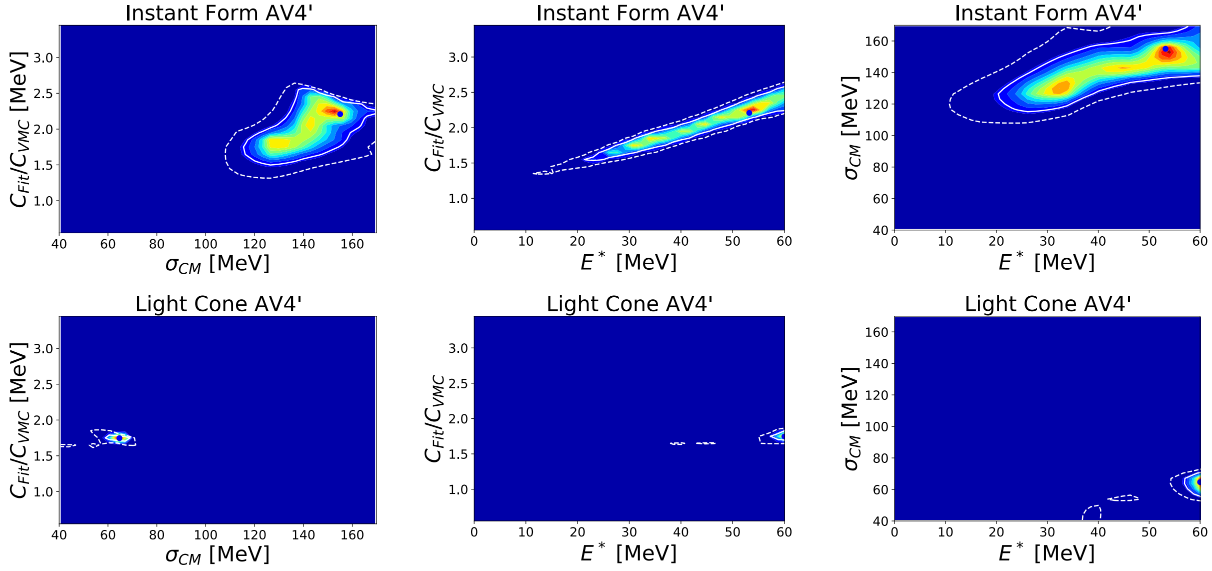


**Fig. S20:** Same as figure 3 for $^{12}$C using the AV4’ potential and the data of Schmookler et al.

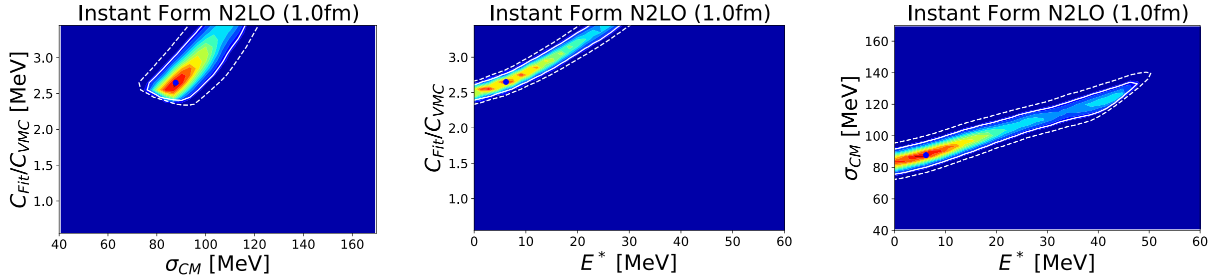

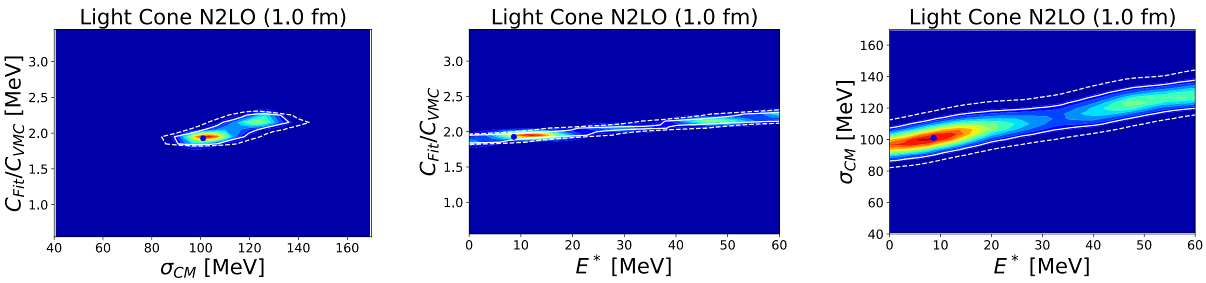


**Fig. S21:** Same as figure 3 for $^{12}C$ using the N2LO(1.0fm) potential and the data of Schmookler et al.

**Best fit GCF calculations compared with data:**

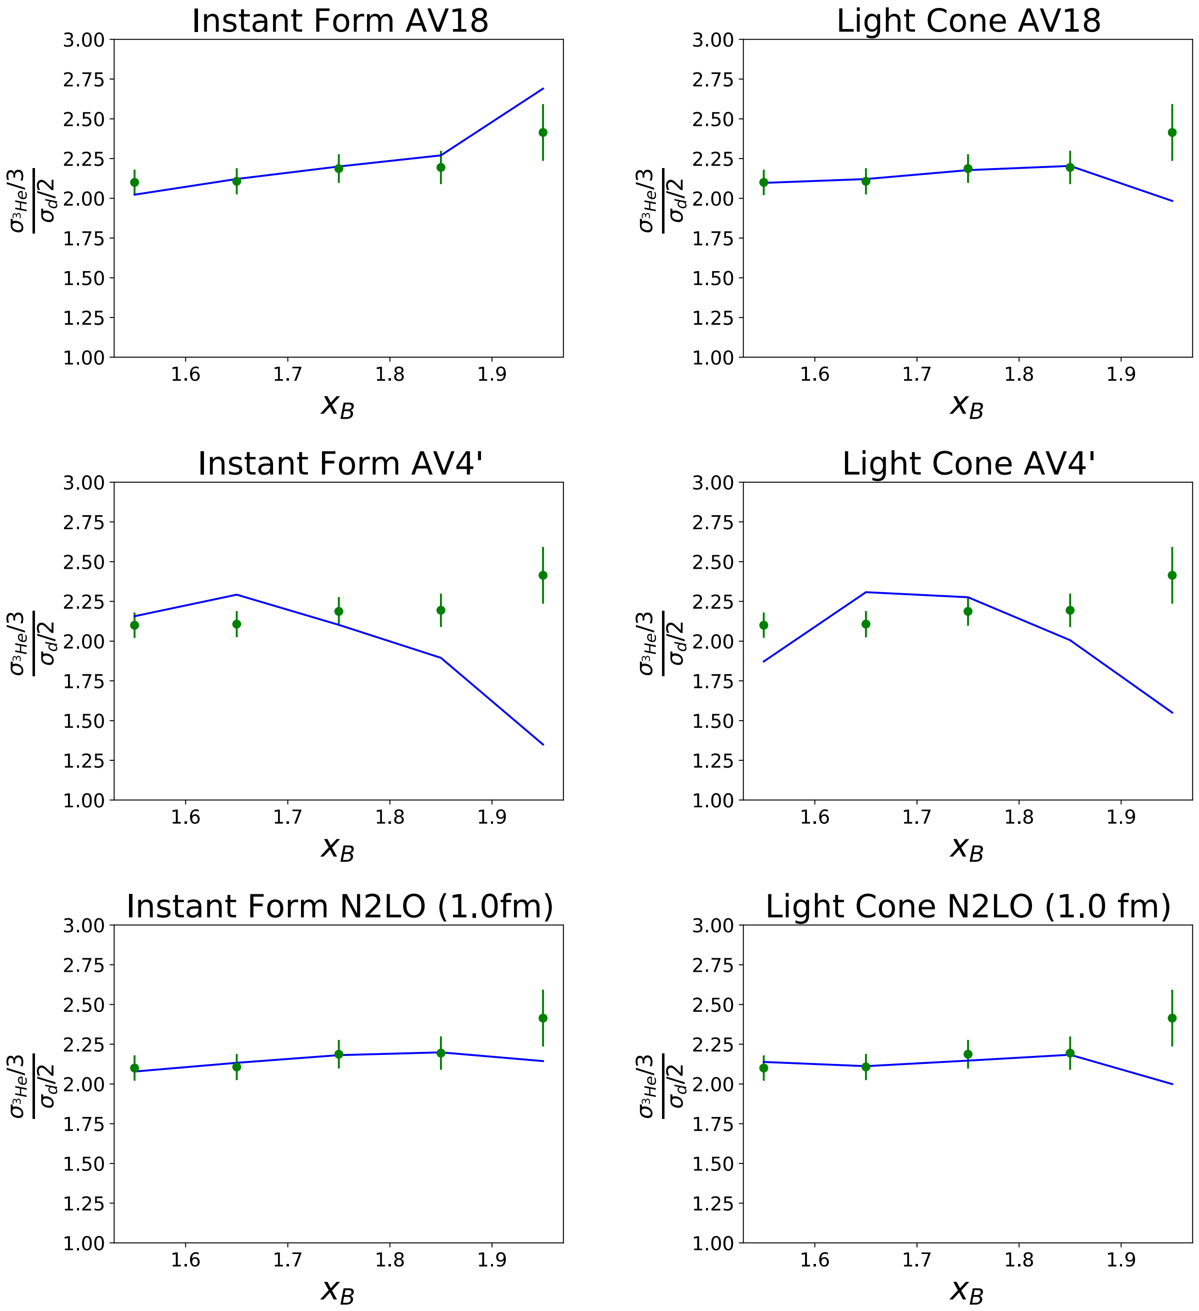

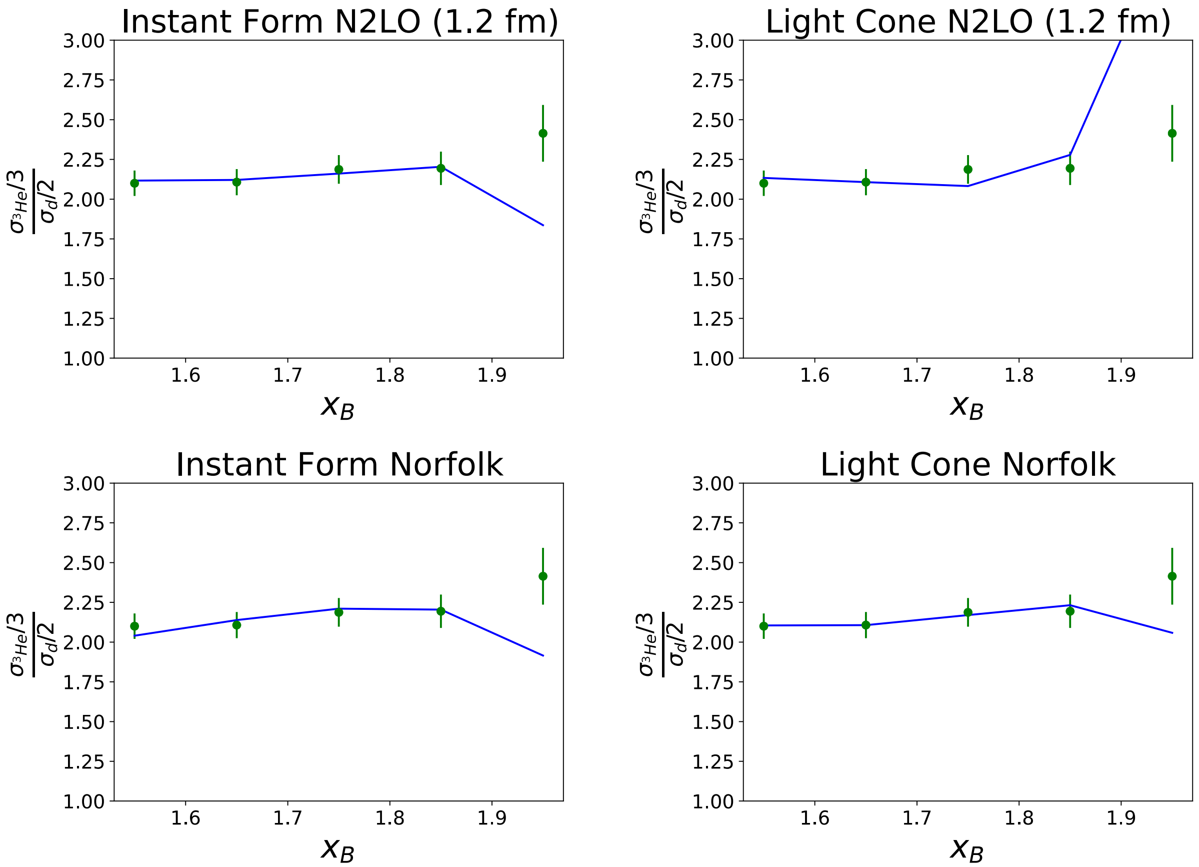


**Fig. S22:** GCF predictions for $^3$He using best fit parameters (table I) using AV18 (top), AV4’, N2LO(1fm), N2LO(1.2fm), Norfolk (bottom) and Instant Form (left) and light-cone (right) formulations.

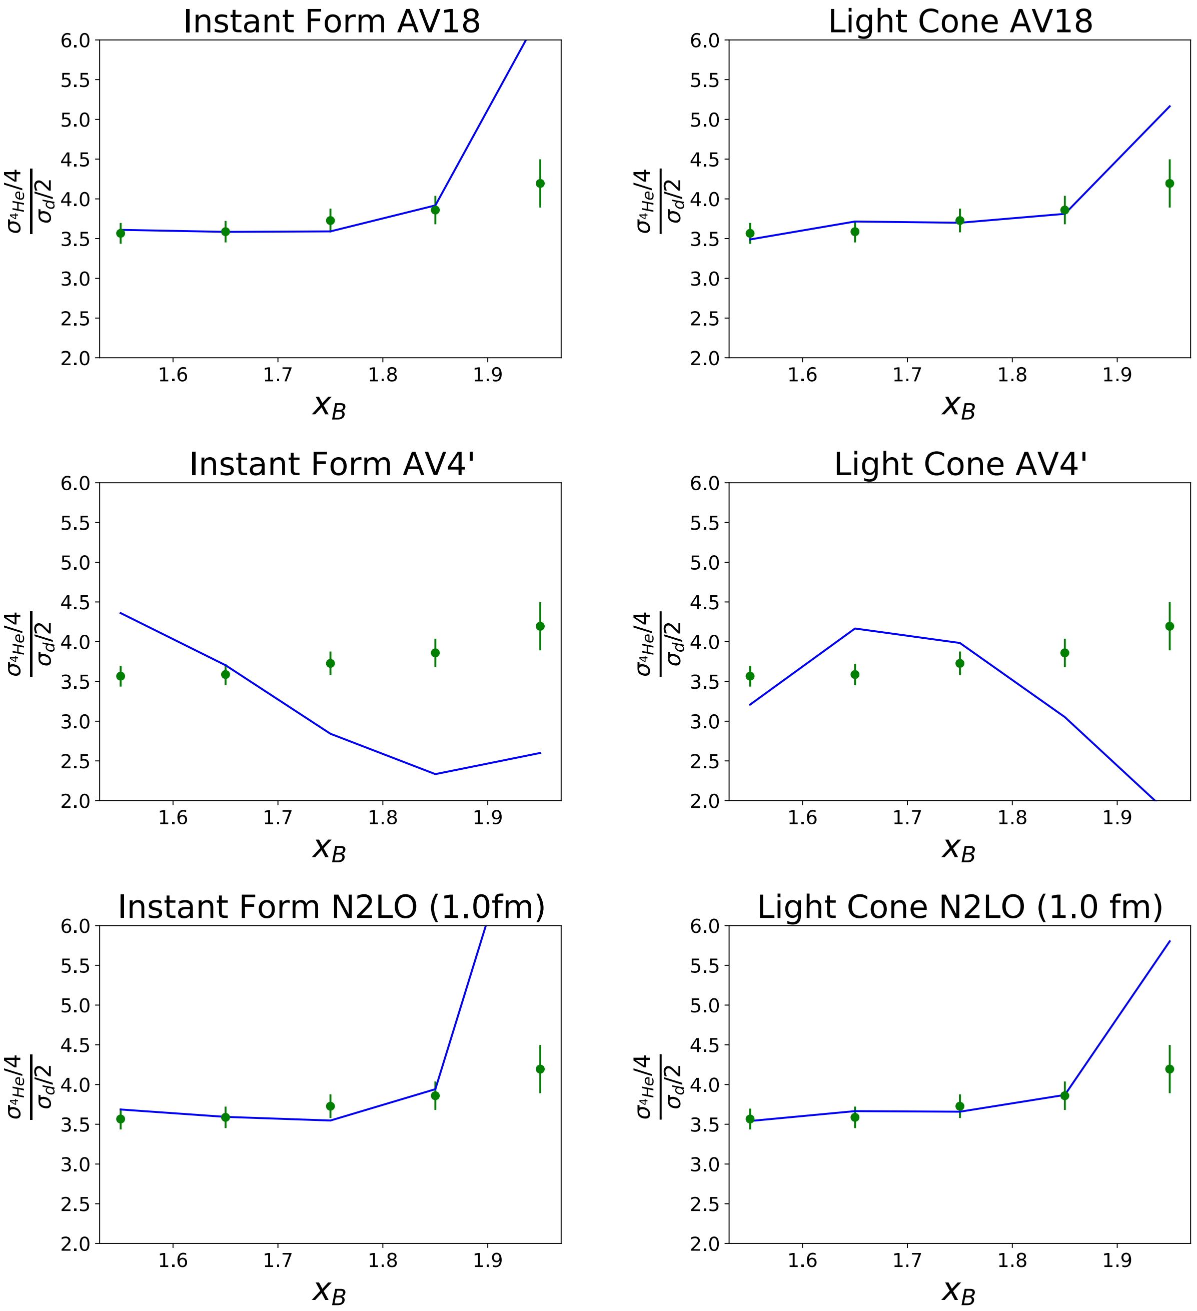

Instant Form AV18
Light Cone AV18
Instant Form AV4'
Light Cone AV4'
Instant Form N2LO (1.0fm)
Light Cone N2LO (1.0 fm)
$\frac{\sigma_{^4He}/4}{\sigma_d/2}$
$x_B$
2.0
2.5
3.0
3.5
4.0
4.5
5.0
5.5
6.0
1.6
1.7
1.8
1.9

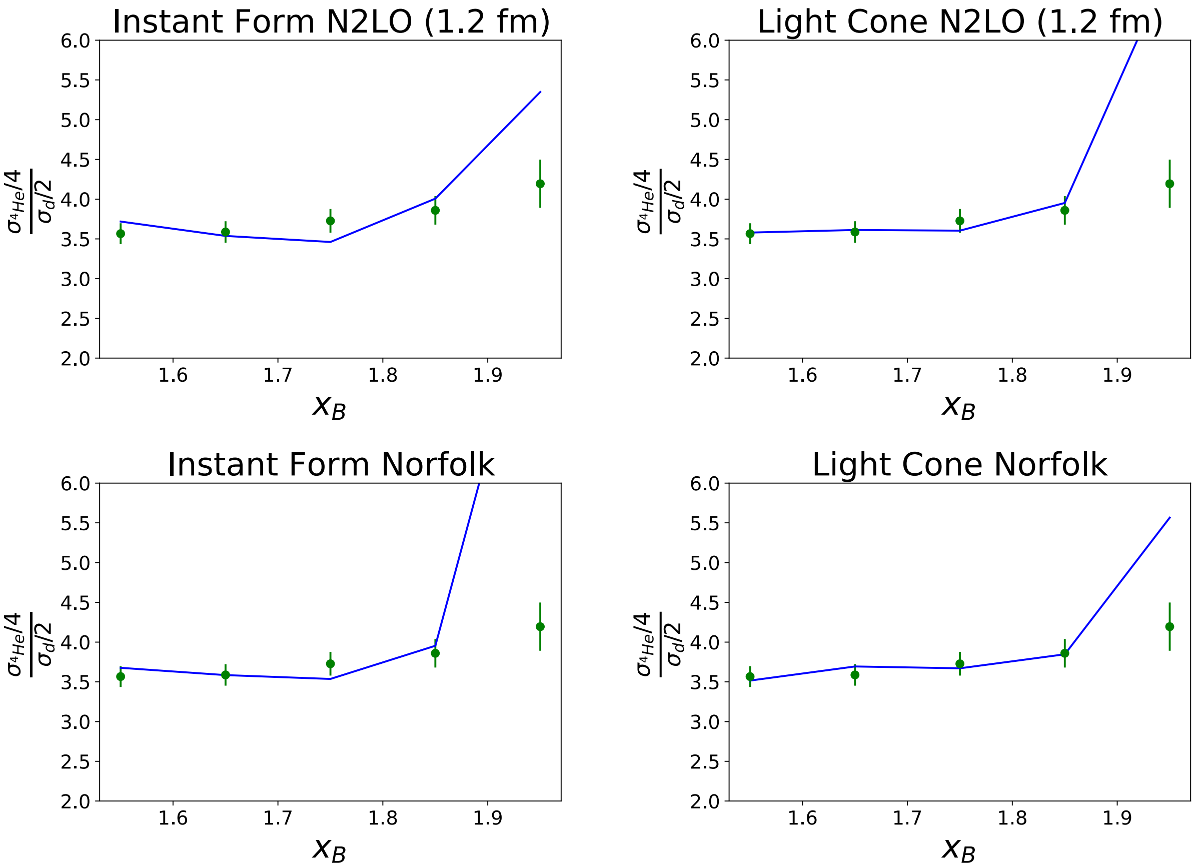


**Fig. S23:** GCF predictions for $^4$He using best fit parameters (table I) using AV18 (top), AV4', N2LO(1fm), N2LO(1.2fm), Norfolk (bottom) and Instant Form (left) and light-cone (right) formulations.

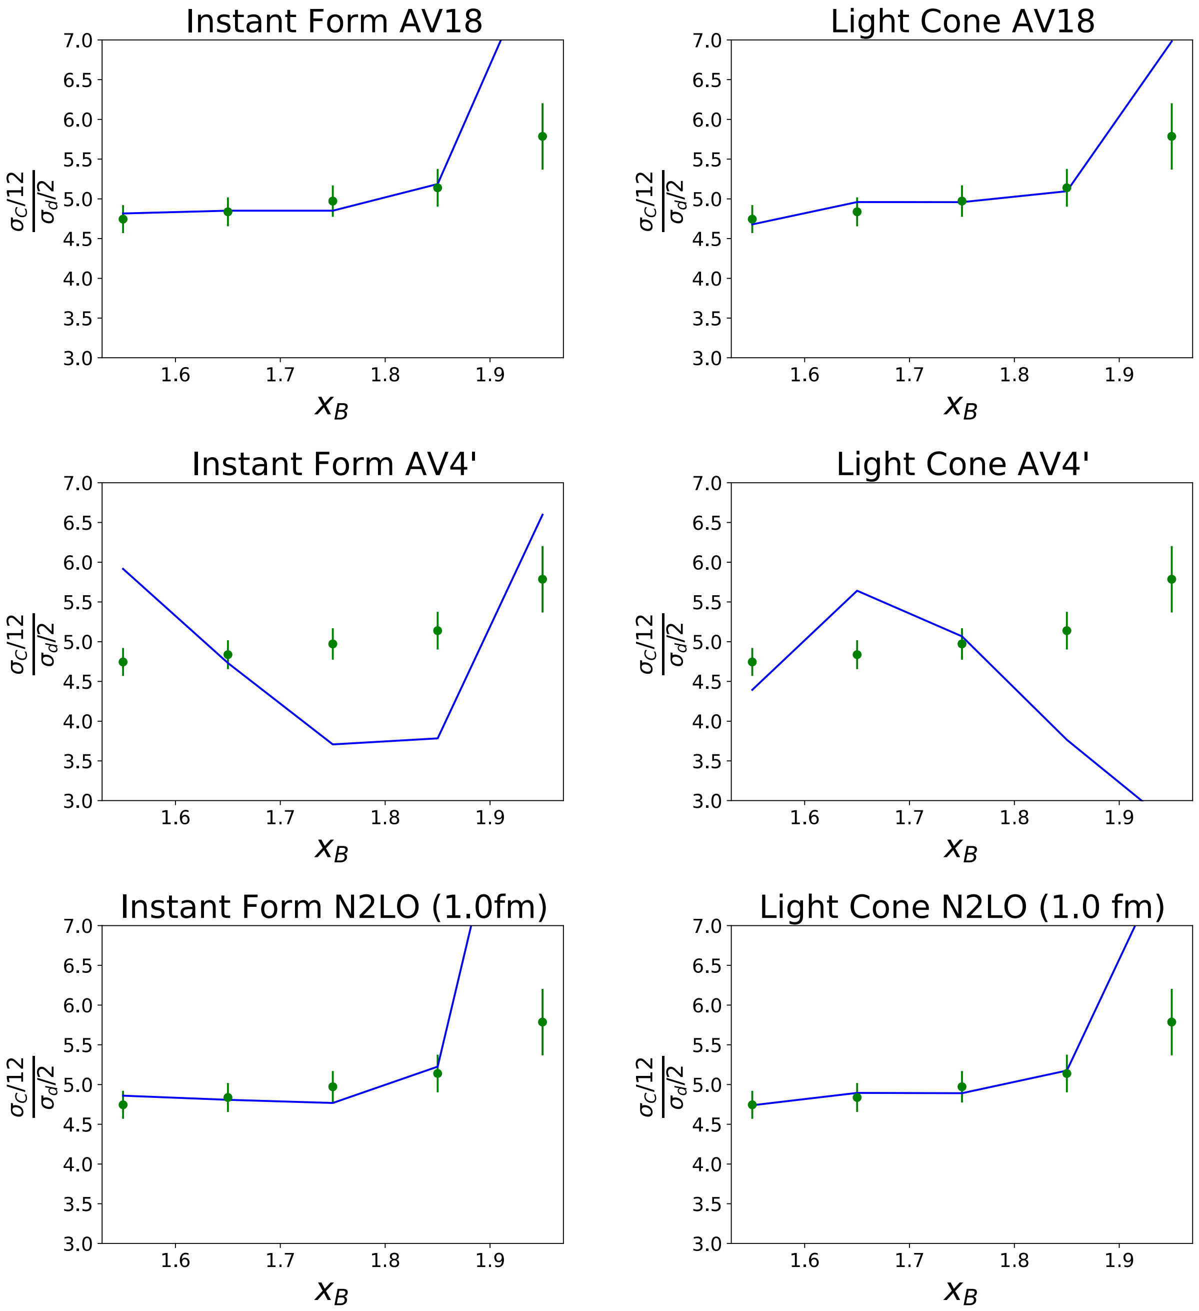


**Fig. S24:** GCF predictions for $^{12}C$ using best fit parameters (table I) using AV18 (top), AV4’, N2LO(1fm) (bottom) and Instant Form (left) and light-cone (right) formulations.

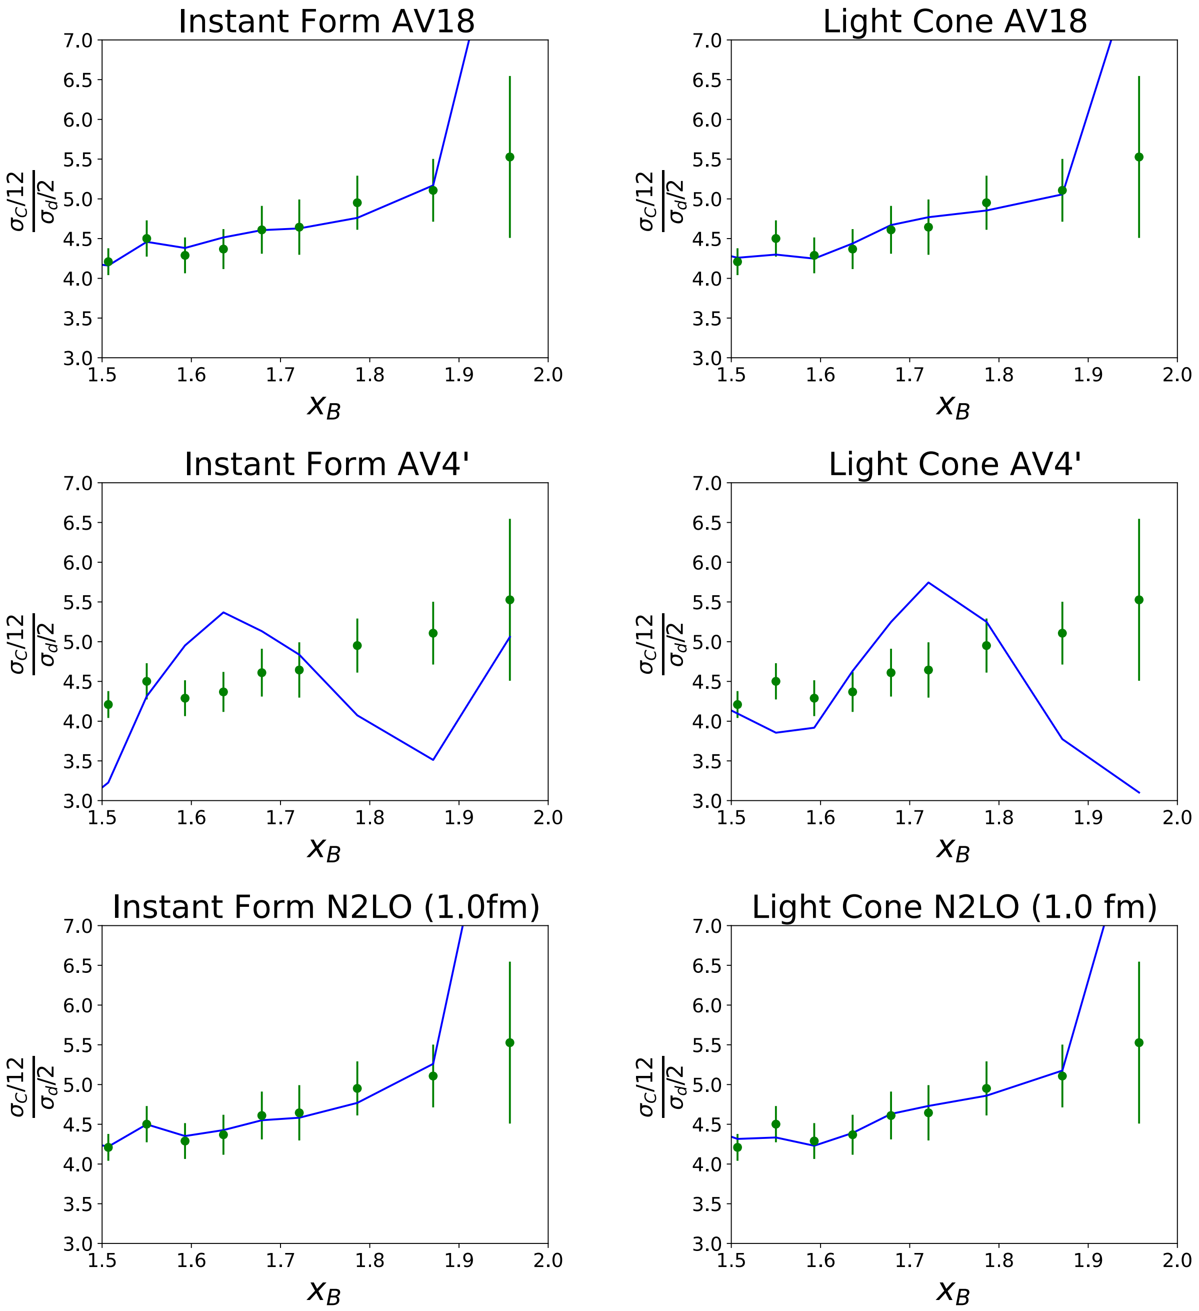


**Fig. S25:** GCF predictions for $^{12}C$ using best fit parameters (table I) using AV18 (top), AV4', N2LO(1fm) (bottom) and Instant Form (left) and light-cone (right) formulations.
